# Supplementary material for: Hierarchical Action Recognition: A Contrastive Video-Language Approach with Hierarchical Interactions
Source: arXiv:2405.17729 source file (2024-05-28)
Supplement: Supplementary file 1 [file X_suppl.tex]

\clearpage
\setcounter{page}{1}
\maketitlesupplementary

\section{Details of Study}
In this section, we show details of FMA dataset and experimental setup in this study.

\subsection{FMA Dataset}
\label{sec:dd}

We present the details of FMA dataset here. Table~\ref{tab:FMA_stat} shows the statistical information of the FMA dataset, as well as the splitting of the training set, validation set and test set in different experiments. Table~\ref{tab:fma_full} shows the overall description of the FMA categories, including four types of assessment items, and three scoring levels under each item. 

\subsection{Experimental Setup}
For the experimental setup, we provide more detailed information on the computational environment and parameter settings.

\noindent \textbf{Computational Environment.}
All experiments are conducted on a server of Ubuntu 20.04.6 LTS (64-bit) with a 13th Gen Intel(R) Core(TM) i7-13700K processor, and a NVIDIA A6000 GPU. We use Python\footnote{https://www.python.org/downloads/release/python-3810/} 3.8.10 for programming and  PyTorch\footnote{https://pytorch.org/} 2.0.0 is used for the learning framework.
\input{tab/FMA_stat}
\input{tab/X_FMA}
\input{tab/setup}
\begin{figure*}[t]
  \centering
   \includegraphics[width=0.98\linewidth]{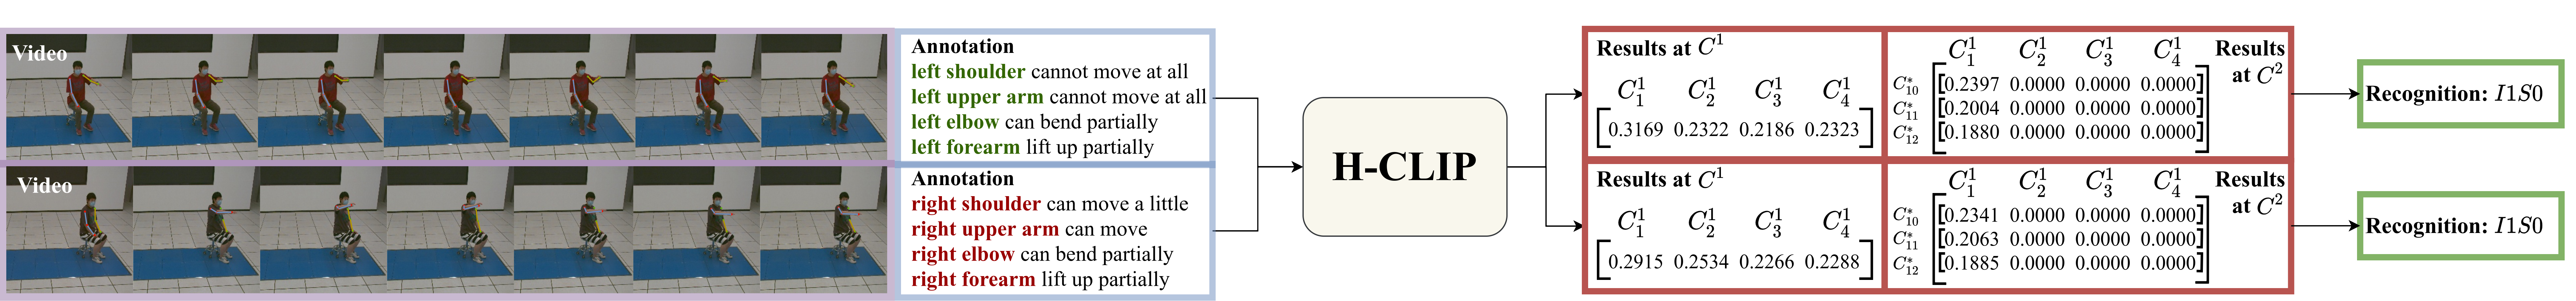}
   \caption{Demonstration of H-CLIP for hierarchical video recognition.}
   \label{fig:demo}
\end{figure*}
\begin{figure}
  \centering
  \begin{subfigure}{0.8\linewidth}
    \includegraphics[width=\linewidth]{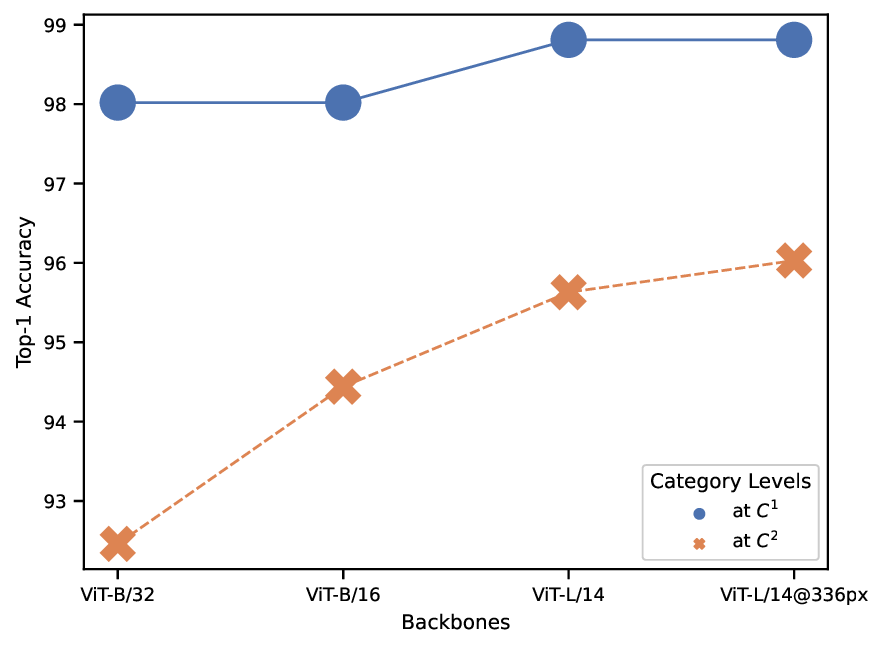}
    \caption{Recognition with different backbones.}
    \label{fig:backbone}
  \end{subfigure}
  \vfill
  \begin{subfigure}{0.8\linewidth}
        \includegraphics[width=\linewidth]{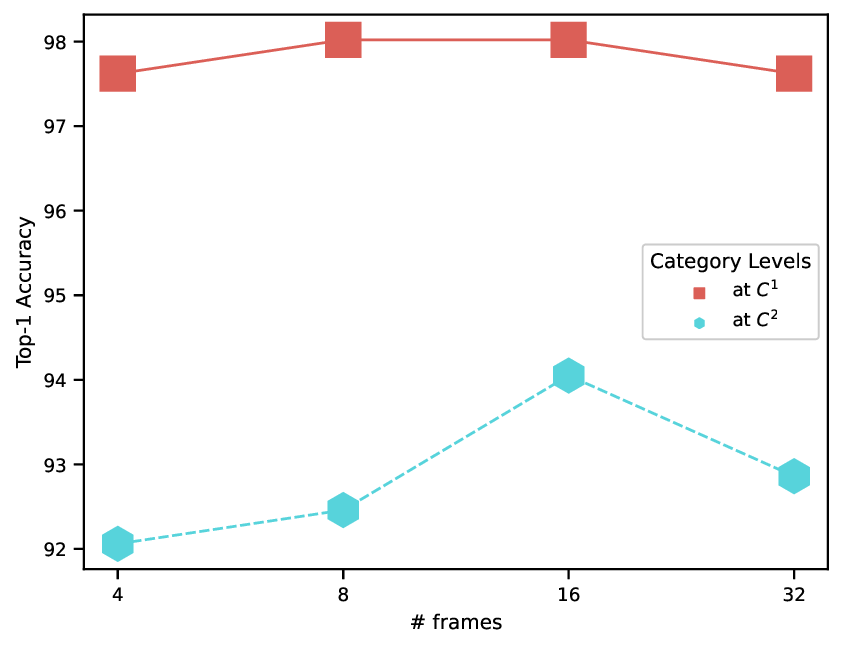}
    \caption{Recognition with different number of frames.}
    \label{fig:frames}
  \end{subfigure}
  \caption{Recognition results of different backbones under 8 video frames as the visual input and different number of frames under ViT-B/32 as the backbone model.}
  \label{fig:bf}
\end{figure}

\noindent \textbf{Parameter Setting.}
Table~\ref{tab:setup} shows the setup of (hyper-) parameters used in all H-CLIP experiments. Parameter settings are the same for all fully supervised learning and few-shot/zero-shot learning experiments.

\section{Detailed Results of Experiments}
In this section, we present the results of some complementary experiments.

\subsection{Demonstration}
Figure \ref{fig:demo} demonstrates hierarchical video recognition using H-CLIP on FMA dataset. The left and right upper limbs are annotatied in the dataset as the text information of videos. The videos and corresponding texts are fed into H-CLIP to produce hierarchical predictions at the $C^1$ and $C^2$ levels (predictions here are indicated by similarity scores between video and category representations). H-CLIP is able to correctly recognize the assessment item at the coarse $C^1$ level, and further refines the fine-grained category at $C^2$. This showcases the capability of our proposed framework for layered hierarchical video understanding.

\subsection{Analysis of Backbones and Number of Frames}
We conduct ablation studies to analyze the impact of backbone architecture and number of input frames on H-CLIP's performance.
Experiments are with varying backbone models including ViT-B/32, ViT-B/16, ViT-L/14 and ViT-L/14@336px under 8 input frames as shown in Figure~\ref{fig:backbone}, which reveal larger backbones consistently improve recognition, especially for fine-grained $C^2$ categories (~3\% gain).
Additional experiments sweeps input frames from 4 to 32 with a ViT-B/32 backbone. Figure~\ref{fig:frames}) demonstrates that the optimal frame number is data-dependent, without a clear universal trend. However, 8 and 16 frames often emerge as prudent choices for video recognition models.
In summary, H-CLIP demonstrates stable $C^1$ recognition across configurations. For the more challenging fine-grained $C^2$ task, performance is sensitive to backbone scale and input frames, but remains highly accurate (92\%+), highlighting the efficacy of our approach.

\section{Discussion}
Unlike mainstream tasks, medical video language understanding demands greater precision, as action differences are often subtle (e.g. $I1S0$ vs $I1S1$, the difference only in that shoulder abduction or elbow flexion occurs "during" or "immediately".). Distinguishing such fine-grained details requires both adequate temporal coverage and precise spatial localization of salient motions. Therefore, a key challenge is accurately predicting assessment items and identifying behavioral differences to determine fine-grained scores given coarse assessments. Our work proposes a contrastive video-language approach with fine-grained attention and hierarchical interaction, demonstrating promising results on this difficult task. However, significant research remains to address the intricate complexities of fine-grained medical video understanding. 
The precise spatio-temporal modeling required stretches the capacities of current methods. Our work provides a stepping stone for medical assessment applications towards uncovering discriminative visual cues and learning representations by hierarchical recognition. Further innovations in architecture, objectives and incorporation of domain knowledge will be essential to fully tackle this emerging and socially impactful challenge.

% \noindent \textbf{Future Work}

{
    \small
    \bibliographystyle{ieeenat_fullname}
    \bibliography{main}
}

% To split the supplementary pages from the main paper, you can use \href{https://support.apple.com/en-ca/guide/preview/prvw11793/mac#:~:text=Delete%20a%20page%20from%20a,or%20choose%20Edit%20%3E%20Delete).}{Preview (on macOS)}, \href{https://www.adobe.com/acrobat/how-to/delete-pages-from-pdf.html#:~:text=Choose%20%E2%80%9CTools%E2%80%9D%20%3E%20%E2%80%9COrganize,or%20pages%20from%20the%20file.}{Adobe Acrobat} (on all OSs), as well as \href{https://superuser.com/questions/517986/is-it-possible-to-delete-some-pages-of-a-pdf-document}{command line tools}.
